# Supplementary material for: Schema for In-Context Learning
Source: arXiv:2510.13905 source file (2026-03-28)
Supplement: Supplementary file 1 [file ablation1.tex]

\section{Ablation Study on the schema activation}
\label{app:abalation_on_schema_activation}

\begin{figure}[H]
  \centering
  \includegraphics[width=\linewidth]{figure/ablation_study.pdf}
  \caption{GPT-4o Mini solving the {\physicsdataset} questions with examples that are {\same}.}
  \label{fig:ablation}
\end{figure}

To further investigate in isolation the effectiveness of schema activation within our framework, we conducted a controlled ablation study comparing four distinct conditions: {\sysname}, {\oneshot}, Schema Only, and Example Schema only.

\subsection{Design and Nature of Ablation Study}

This ablation analysis was designed to determine whether the performance improvements observed in {\sysname} stem from the schema activation mechanism itself or merely from the presence of abstracted examples. In particular, we are interested in the case when prior examples are of high quality, and therefore conducted this study by using GPT-4o Mini to solve questions in the {\physicsdataset} subset with prior examples that are {\same} in terms of synthetic similarity. The Schema Only condition provided models with abstract problem schemas without corresponding episodic examples, while Example Schema Only presented abstracted schemas derived from examples but without the schema activation process that is integral to the full {\sysname} procedure.

\subsection{Interpretation of Ablation Results}

\Cref{fig:ablation} presents the comparative accuracy results across all four scenarios. The complete {\sysname} framework demonstrated clear superiority over the other three approaches, with a near 40\% accuracy boost over the other three conditions. In fact, neither Schema Only nor Example Schema Only results in a clear benefit over {\oneshot}, which acts as a baseline for this ablation study. This observation provides direct evidence that the schema activation mechanism constitutes the critical component driving the effectiveness of our {\ICL} framework.

\subsection{{\SchemaDormancy}}

The results of our ablation study strongly suggest that the mere presence of an abstracted schema within the prompt context is insufficient to improve model performance. The sheer significance of schema activation leads to a phenomenon which we coin \textit{{\SchemaDormancy}}. This term describes a state where a refined schema tailored to a specific task only exists as passive surface-level contextual information rather than an active cognitive framework that guides the language model's reasoning process. When the explicit activation step of the {\sysname} framework is omitted --- as observed in the Schema Only and Example Schema Only conditions --- the LLM fails to effectively integrate the abstracted reasoning structure into its problem-solving approach. This finding highlights that language models do not implicitly adopt and utilize abstract schemas without an explicit technique to activate this otherwise dormant state.
