# Supplementary material for: Schema for In-Context Learning
Source: arXiv:2510.13905 source file (2026-03-28)
Supplement: Supplementary file 2 [file GPT5.tex]

% \section{GPT-5's Performance on Humanity's Last Exam}
% \label{app:gpt5}
% While we focused mostly on smaller models, we believe it's worth showing the results of a larger model on an even more challenging dataset, to better justify the usage of {\sysname} beyond smaller models. Here, we reported the result of using {\sysname} with GPT-5 on HLE subsets in \Cref{fig:gpt5}.
% \begin{figure}[h!]
%   \centering
%   \includegraphics[width=\linewidth]{figure/hle.pdf}
%   \caption{Performance of GPT-5 on the chemistry, physics, biology multi-choice questions from the Humanity's Last Exam (HLE) benchmark dataset \citep{phan2025humanity} (N=191, we filtered out questions with images), when provided with the {\same} examples. We generated the synthetic data as well using the same procedures described in \Cref{app:synthetic_data_generation}.}
%   \label{fig:gpt5}
% \end{figure}

% When GPT-5 was introduced, we used the model to run the same experiments. However, we realized that when provided with {\same} examples, GPT-5 reached near 100\% accuracy in the GPQA dataset, eliminating the need for explicit reasoning modules introduced by {\sysname}. Therefore, we used a more challenging dataset, Humanity's Last Exam (HLE), to repeat the same experiments using {\same} examples, and saw that {\sysname} results in a 7\% improvement in accuracy compared to standard {\oneshot}. This gain is particularly notable given the already strong baseline accuracy of 84\%.

% Note that this subset of HLE includes 136 biology and medicine questions, 34 physics questions, and 21 chemistry questions. We acknowledge that most of the questions are in the biology and medicine sub-categories, which is a domain that was not tested in the main experiments shown in \Cref{tab:full_results}.
